# Supplementary material for: A simple and efficient convex optimization based bound-preserving high order accurate limiter for Cahn-Hilliard-Navier-Stokes system
Source: arXiv:2307.09726 source file (2024-03-29)
Supplement: Supplementary file 1 [file appendix.tex]

\section{High-order accuracy of the cell average limiter}\label{sec:appendix}
In the context of the DG scheme, the high order accurate cell average limiter that preserves conservation and bounds can be formulated as seeking a piecewise constant polynomial $x_h$ solving
\begin{equation}\label{eq:appendix:opt_model1}
\min_{x_h} \norm{x_h - \overline{u_h}}{L^2}^2 \quad\mathrm{s.t.}\quad
\int_\Omega x_h = \int_\Omega u_h ~~\text{and}~~ m \leq x_h\leq M.
\end{equation}
Here, the $\overline{u_h}$ is a piecewise constant polynomial that value on each cell $E$ equals the cell average of $u_h$, namely $\on{\overline{u_h}}{E} = \frac{1}{\abs{E}}\int_E u_h$. We denote the solution of the minimization problem \eqref{eq:appendix:opt_model1} by $\overline{w_h}$. Then, the postprocessed polynomial  
\begin{equation}\label{eq:appendix:opt_model1_post}
u_h^\mathrm{lim} = (u_h - \overline{u_h}) + \overline{w_h}
\end{equation}
preserves conservation and bounds of cell average. Let us prove the modification \eqref{eq:appendix:opt_model1_post} is of the same approximation order to the exact solution $u$.
\par
Construct a polynomial $\mathcal{P}_h u$ by taking $L^2$ projection of the exact solution $u$ then applying the Zhang--Shu limiter. Thus, the polynomial $\mathcal{P}_h u$ is an approximation of $u$ that satisfies $\norm{\mathcal{P}_h u - u}{L^2} \leq Ch^{k+1}$ and $m \leq \mathcal{P}_h u \leq M$.
Let $\overline{\mathcal{P}_h u}$ denote a piecewise constant polynomial that value on each cell equals the cell average of $\mathcal{P}_h u$. It is straightforward to verify $m \leq \overline{\mathcal{P}_h u} \leq M$. Since the $L^2$ projection, the Zhang--Shu limiter, and the numerical scheme preserve conservation, we have
\begin{equation*}
\int_\Omega \overline{\mathcal{P}_h u} 
%= \sum_{E\in \setE_h} \int_E \overline{\mathcal{P}_h u} 
= \sum_{E\in \setE_h} \int_E \Big(\frac{1}{\abs{E}}\int_E \mathcal{P}_h u\Big) 
%= \sum_{E\in \setE_h} \int_E \mathcal{P}_h u
= \int_\Omega \mathcal{P}_h u
= \int_\Omega u
= \int_\Omega u_h.
\end{equation*}
By \eqref{eq:appendix:opt_model1_post}, the postprocessed polynomial satisfies $u_h^\mathrm{lim} - u_h = \overline{w_h} - \overline{u_h}$. Use triangle inequality and \eqref{eq:appendix:opt_model1}, we have
\begin{equation*}
\norm{u_h^\mathrm{lim} - u}{L^2} 
\leq \norm{\overline{w_h} - \overline{u_h}}{L^2} + \norm{u_h - u}{L^2}
\leq \norm{\overline{\mathcal{P}_h u} - \overline{u_h}}{L^2} + \norm{u_h - u}{L^2}.
\end{equation*}
Thus, if the numerical solution $u_h$ is optimal in $L^2$ norm, then we only need to show $\norm{\overline{\mathcal{P}_h u} - \overline{u_h}}{L^2}\leq Ch^{k+1}$. Actually, this is guaranteed by Cauchy--Schwarz's inequality. We have
\begin{align*}
\norm{\overline{\mathcal{P}_h u} - \overline{u_h}}{L^2}
&= \sum_{E\in \setE_h} \norm{\frac{1}{\abs{E}}\int_E (\mathcal{P}_h u - u_h)}{L^2(E)}\\
&\leq \sum_{E\in \setE_h} \frac{1}{\abs{E}} \norm{\mathcal{P}_h u - u_h}{L^2(E)} \norm{1}{L^2(E)}^2 
= \norm{\mathcal{P}_h u - u_h}{L^2}.
\end{align*}
We conclude the proof since $\norm{\mathcal{P}_h u - u_h}{L^2} \leq \norm{\mathcal{P}_h u - u}{L^2} + \norm{u_h - u}{L^2} \leq Ch^{k+1}$.
